# Supplementary material for: AlignFreeze: Navigating the Impact of Realignment on the Layers of Multilingual Models Across Diverse Languages
Source: arXiv:2502.12959 source file (2025-02-18)
Supplement: Supplementary file 1 [file original_appendix_tables.tex]

\begin{table*}[!h]
\centering
\resizebox{\textwidth}{!}{%
% [inline block 0: 12 envs, 87143 chars -> data_tex | \begin{tabular}{@{}cccccccccccccc@{}} \toprule...]

\caption{NLI average accuracy results across 5 seeds using distilMBERT for the freeze methods by language, training approach, and aligner. The dataset is filtered to the 50th percentile using QE values. Aligner names: FA - FastAlign, AA - AwesomeAlign, BD - Bilingual Dictionaries. The highest average accuracy value for each language is highlighted in bold.}
\label{table:nli_results_distilmbert_50th_qe_percentile}
\end{table*}
